# Supplementary material for: Comfort energy management system for electrified buildings using hydrogen for seasonal storage
Source: arXiv:2511.04293 source file (2026-11-19)
Supplement: Supplementary file 1 [file 05_supplementaries.tex]

%\appendix

\section{Mathematical models}
\label{sec:appendix_models}

This supplementary section describes the models used for evaluating the scenarios. 
Subsections \ref{sec:Photovoltaic} and \ref{sec:Battery} describe the \ac{PV} generation and \ac{BESS}, respectively. The hydrogen system composed of the fuel cell and hydrogen storage is described in Section \ref{sec:h2}. Sections \ref{sec:hp} and \ref{sec:dhw} follow with the description of the heat pump energy conversion and domestic hot water storage system. Finally, to exploit the thermal building flexibility, the building model is described in Section \ref{sec:bldg}.
Moreover, after each model description, model assumptions are provided. 

%Introduced sets: $\forall k \in \mathcal{K}$
%%%%%%%%%%%%%%%%%%%%%%%%%%%%%%%%%%%%%%%%%%%%%%%%%%
\subsection{\acl{PV} (\acs{PV})}
\label{sec:Photovoltaic}
\ac{PV} generation defined in existing literature \cite{al2019home} is outlined with the Equation \eqref{eq:power_pv}.
It is subject to the number of modules $n_\mathrm{module}$, the area of each module $a_\mathrm{module}$ in $\si{\meter ^2}$ and the incident solar radiation falling on the tilted module $G_k$ in the time step $k$ calculated in $\si{\watt/\meter ^2}$. The incident solar radiation $G_k$ is calculated based on global radiation $\dot{q}_\mathrm{s}$, diffuse solar radiation, and tilted angle \cite{hazyuk2012optimal}. 
The $NOCT$ represents the nominal operating cell temperature, $T_{\mathrm{amb},k}$ is the ambient air temperature, and $T_\mathrm{STC}$ is the temperature under the standard testing conditions. All three are defined in \si{\degree C}. 
The \ac{PV} generation is given by the following equation:

\begin{align}
    P_{\mathrm{PV},k} &= n_\mathrm{module}\cdot a_\mathrm{module}\cdot G_k\cdot \eta_\mathrm{STC}\cdot \eta_\mathrm{L\&T}\cdot \Bigl[1-\bigl(\eta_T \cdot (T_{\mathrm{amb},k} + \frac{NOCT-20\si{\celsius}}{800\si{\watt/\meter^2}} \cdot G_k-T_\mathrm{STC})\bigr)\Bigr],\label{eq:power_pv}
\end{align}

where the term $(NOCT-20\si{\celsius})/800\si{\watt/\meter^2}$ represents the overall heat loss coefficient in $\si{\celsius/(\watt/\meter^2)}$ \cite{rouhani2013comprehensive}. Besides that, the power generated $P_{\mathrm{PV},k}$ depends on the following efficiencies $\eta_\mathrm{STC}$ representing the electrical efficiency of the PV module at standard testing conditions, $\eta_\mathrm{L\&T}$ accounting for the combined energy losses associated with the inverter and the maximum power point tracking controller, and the temperature coefficient  $\eta_T$ in $\si{1/\degree C}$ of PV generation.

The \ac{PV} generation depends on ambient air temperature and incident solar radiation, assuming linear photovoltaic behavior, and neglecting dynamic electrical behavior. % IV (current–voltage) characteristics
Furthermore, the degradation over time and shading losses are also neglected.



%%%%%%%%%%%%%%%%%%%%%%%%%%%%%%%%%%%%%%%%%%%%%%%%%%
\subsection{\acl{BESS} (\acs{BESS})}
\label{sec:Battery}

Battery energy state SOC$_k$ at time step $k$, from \cite{javadi2020optimal}, depends on the previous state SOC$_{k-1}$, the charging and discharging power $P_{\mathrm{ch},k}$ and $P_{\mathrm{d},k}$, respectively, the efficiency of the charging and discharging processes $\eta_\mathrm{ch}$ and $\eta_\mathrm{d}$, respectively, and the maximum battery capacity $E_\mathrm{B,max}$: 
\begin{align}
    \text{SOC}_k &= \text{SOC}_{k-1} + \frac{\eta_\mathrm{ch} \cdot P_{\mathrm{ch},k} \cdot t_\mathrm{s} - \frac{P_{\mathrm{d},k}}{\eta_\mathrm{d}}\cdot t_\mathrm{s}}{ E_\mathrm{B,max}},\label{eq:batt_soc} 
\end{align}
where the parameter $t_\mathrm{s}$ indicates sample time in hours.

The linear dependence between charging and discharging processes and the battery's \acs{SOC} is assumed. 
The effect of \ac{BESS} self-discharge is not considered.

\ac{BESS} is constrained by Equations (\ref{eq:SOC_const}) and (\ref{eq:bat_ch_dis_const}). The binary variables $s_{\mathrm{ch},k}$ and $s_{\mathrm{d},k}$, defined with Equations (\ref{eq:s_binary}) and (\ref{eq:s_summ}), are employed to restrict charging and discharging concurrently. 
Accordingly, \ac{BESS} can operate in one of three mutually exclusive modes at each time step: charging ($s_{\mathrm{ch},k}=1$, $s_{\mathrm{d},k}=0$), discharging ($s_{\mathrm{ch},k}=0$, $s_{\mathrm{d},k}=1$), or remaining idle ($s_{\mathrm{ch},k}=0$, $s_{\mathrm{d},k}=0$):

\begin{align}
    \text{SOC}_\mathrm{min} \le &\text{SOC}_k \le \text{SOC}_\mathrm{max}, \label{eq:SOC_const}  \\
    s_{c,k} \cdot P_{c,\mathrm{min}} \le &P_{c,k} \le s_{c,k} \cdot P_{c,\mathrm{max}},\label{eq:bat_ch_dis_const}\\
    s_{\mathrm{c},k} \in \{0,1\} \label{eq:s_binary};& \quad
    \forall c \in \{\mathrm{ch},\mathrm{d}\}, \\
    s_{\mathrm{ch},k} &+ s_{\mathrm{d},k} \in \{0,1\}. \label{eq:s_summ}
\end{align}


%%%%%%%%%%%%%%%%%%%%%%%%%%%%%%%%%%%%%%%%%%%%%%%%%%
\subsection{Hydrogen system}\label{sec:h2}
%%%%%%%%%%%%%%%%%%%%%%%%%%%%%%%%%%%%%%%%%%%%%%%%%%

Green hydrogen, ideally generated in summer using an electrolyzer when \ac{RES} generation exceeds the demand, is stored in the hydrogen storage.
In winter, when demand is high, the hydrogen is converted back into electricity using a fuel cell. 
Because the fuel cell generates heat as a byproduct, it is used as a cogeneration utility, where the heat is recovered and used to meet domestic hot water demand. 
The hydrogen system, consisting of \ac{PEMFC} and hydrogen storage, is modeled and parametrized in accordance with the existing literature \cite{cheng2025multi,wang2025dynamic,nondy20244e}. 
\ac{PEMFC} is hereafter referred to as the fuel cell.

The voltage of the single cell is defined by the Nernst open-circuit voltage $E_\mathrm{Nernst}$ and activation polarization $V_\mathrm{act}$, ohmic polarization $V_\mathrm{ohm}$, and concentration polarization $V_\mathrm{con}$ loss voltages measured in \si{\volt}:
\begin{align}
    V_{\mathrm{cell},k} = E_{\mathrm{Nernst}}(I_{\mathrm{FC},k}) - V_{\mathrm{act}}(I_{\mathrm{FC},k}) - V_{\mathrm{ohm}}(I_{\mathrm{FC},k}) - V_{\mathrm{con}}(I_{\mathrm{FC},k}),
\end{align}
where each term is a function of stack current $I_\mathrm{FC}$ measured in \si{\ampere}. 
The voltages are modeled according to \cite{cheng2025multi}, which provides a comprehensive description with empirical parameter identification.
The stack power of the fuel cell is then calculated as:
\begin{align}
P_{\mathrm{FC},k} = n_\mathrm{cell} \cdot V_\mathrm{cell}(I_{\mathrm{FC},k})\cdot I_{\mathrm{FC},k},
\end{align}
where $n_\mathrm{cell}$ represents the number of cells in the stack.
The molar hydrogen flow consumption, measured in \si{\mol/\second} is calculated as follows:
\begin{align}
\dot{n}_{\mathrm{FC},k} = \beta \cdot \frac{n_\mathrm{cell}\cdot I_{\mathrm{FC},k}}{2\cdot F},
\end{align}
where $\beta$ represents the stoichiometric rate of hydrogen, and $F$ is Faraday constant measured in \si{\coulomb/\mol}.
The heat recovery is defined as follows:
\begin{align}
\dot{Q}_{\mathrm{hr},k} = \dot{n}_{\mathrm{FC},k}\cdot \text{LHV}\cdot \eta_\mathrm{FC,sys} - P_{\mathrm{FC},k},
\end{align}
where LHV represents the lower heating value of hydrogen in \si{\joule/\mol} and $\eta_\mathrm{FC,sys}$ system efficiency of the fuel cell.
Analogously to the \ac{BESS}, the \ac{LOH} in the storage is calculated as the energy content of hydrogen in the storage: 
\begin{align}
    \text{LOH}_k &= \text{LOH}_{k-1} -\frac{\dot{n}_{\mathrm{FC},k} \cdot \text{LHV} \cdot t_\mathrm{s}}{ E_\mathrm{H_2,max}}.
    \label{eq:LOH}
\end{align}

\ac{LOH} depends on the previous state and the hydrogen consumed at the current time step.
The system is constrained by:
\begin{align}
    \text{LOH}_\mathrm{min} &\le \text{LOH}_k \le \text{LOH}_\mathrm{max}, \\
    I_{\mathrm{FC},\mathrm{min}} &\le I_{\mathrm{FC},k}\le  I_{\mathrm{FC},\mathrm{max}}, 
\end{align}
where hydrogen storage is restricted by minimal LOH$_\mathrm{min}$ and maximal LOH$_\mathrm{max}$ level of the hydrogen in the storage. 
The fuel cell is constrained by corresponding minimal $I_{\mathrm{FC},\mathrm{min}}$ and maximal $I_{\mathrm{FC},\mathrm{max}}$ stack current. 
Figure \ref{fig:fuel_cell_performance} presents the cell voltage, efficiency, fuel cell stack power, and generated heat related to current density. 
The gray area represents the fuel cell operating zone, within which the power output of the fuel cell is approximated by a linear model.

\begin{figure}[h!]
    \centering
    \includegraphics[width=0.7\textwidth]{figures/fuel_cell_performance.pdf}
    \caption{The fuel cell performance based on the model from \cite{cheng2025multi}. The gray area represents the fuel cell operating zone.}
    \label{fig:fuel_cell_performance}
\end{figure}

Current density is defined as follows: 
\begin{align}
    i_{\mathrm{FC},k} = \frac{I_{\mathrm{FC},k}}{a_\mathrm{cell}}, 
\end{align}

where $a_\mathrm{cell}$ represents the effective activation area of a single cell.
The linear power approximation is used in \ac{MPC} as a linear fuel cell model, where the current is the control signal.

This model assumes steady-state operation and uses the ideal gas law.
The fuel cell temperature is kept constant at 65\,\si{\celsius}.
Moreover, we assume a constant fuel cell system efficiency of 75\% for heat-recovery evaluation, according to the literature \cite{gandiglio2014design, ellamla_current_2015, nguyen_proton_2020}.
Ideally, the electrolyzer produces green hydrogen in summer, and the hydrogen is stored at lower pressures, such as 13.8--30\,\si{\bar} \cite{cau2014energy, acar2023performance}. 
When producing hydrogen, there would be no additional losses due to compression, as the electrolyzer can compress hydrogen to the above-mentioned pressure levels \cite{acar2023performance}.
Since this work focuses on efficient hydrogen use in winter, the electrolyzer is out of scope and therefore not modeled.




%%%%%%%%%%%%%%%%%%%%%%%%%%%%%%%%%%%%%%%%%%%%%%%%%%
\subsection{Heat pump}
\label{sec:hp}
The heat pump is modeled to transform electrical power $P_{\mathrm{HP}}$ into heat flow $\dot{Q}_{\mathrm{h}}$, which is subsequently utilized for space heating or domestic hot water. The \ac{COP} and maximal electricity power intake $P_\mathrm{HP, max}$ are contingent on the ambient air temperature $T_\mathrm{amb}$ and supply water temperature, which is either  55\,\si{\degree C}  for space heating or 45\,\si{\degree C} for domestic hot water. The modulation factor $\eta_\mathrm{HP}$ dictates the electrical power intake of the heat pump and is controlled by \ac{EMS}. It is constrained to be either between 0.2 and 1, or the heat pump is turned off. 
The equations describing the model are as follows:
\begin{align}
    \dot{Q}_{{\mathrm{h}},k} = \text{COP}_k \cdot P_{\mathrm{HP},k},& \quad  \text{COP}_k = \text{COP}(T_{\mathrm{amb},k}, T_{\mathrm{supply},k}),\\
    P_{\mathrm{HP},k} = \eta_{\mathrm{HP},k} P_{\mathrm{HP, max},k},& \quad \eta_{HP} \in {\{0, [0.2,1]\}}.
\end{align}

Whether the thermal energy is allocated to domestic hot water production or space heating is determined by the \ac{EMS} according to the following equations: 
\begin{align}
   s_{\mathrm{SH},k}\text{ , } s_{\mathrm{DHW},k} \in \{0,1\}, &\quad 
   s_{\mathrm{SH},k} + s_{\mathrm{DHW},k} \in \{0,1\}, \label{eq:hp_binaryVariables}\\
   \dot{Q}_{{\mathrm{h,SH}},k} = s_{\mathrm{SH},k}\dot{Q}_{{\mathrm{h}},k}, & \quad
   \dot{Q}_{{\mathrm{h,DHW}},k} = s_{\mathrm{DHW},k}\dot{Q}_{{\mathrm{h}},k},\label{eq:heat_flux_DHW}
\end{align}
where the binary operator  $s_\mathrm{SH}$ is set to 1 when heating is employed for space heating, and $s_\mathrm{DHW}$ is set to 1 when a heat pump is employed for domestic hot water, without permitting both to be utilized synchronously.

The steady-state performance of the heat pump model is assumed.
Dynamic effects, start-up and shut-down losses, auxiliary electricity consumption, and detailed refrigerant-cycle behavior are neglected.

%%%%%%%%%%%%%%%%%%%%%%%%%%%%%%%%%%%%%%%%%%%%%%%%%%
\subsection{Domestic hot water storage}
\label{sec:dhw}
The domestic hot water storage is modeled using the energy difference equation \cite{dengiz2019demand}:   
\begin{align}
 V_{\mathrm{DHW},k} &= V_{\mathrm{DHW},k-1} + \frac{\dot{Q}_{\mathrm{DHW},k}-\dot{Q}_{\mathrm{dm,DHW},k}-\dot{Q}_\mathrm{l,DHW}}{\Delta T_\mathrm{DHW}\cdot \rho_\mathrm{H_2O} \cdot c_\mathrm{H_2O}}\cdot t_\mathrm{s},\label{eq:DHW_model}
\end{align}

assuming the constant temperature $T_\mathrm{DHW}=\mathrm{const.}$, while the usable volume of the storage $V_\mathrm{DHW}$ in $\si{m^3}$ is subject to variation. 
The $\Delta T_\mathrm{DHW}$ describes the difference between the desired water $T_\mathrm{DHW}$ and the tap water temperature. 
The parameters $\rho_\mathrm{H_2O}$ and $c_\mathrm{H_2O}$ are the density and specific heat capacity of the water, respectively. 
The domestic hot water demand is denoted by $\dot{Q}_\mathrm{dm,DHW}$ and the standing losses by $\dot{Q}_\mathrm{l,DHW}$. 
The total heat flow $\dot{Q}_\mathrm{DHW}$ entering the system is the sum of the heat flows from the heat pump and the heat recovered from the fuel cell:
\begin{align}
 \dot{Q}_{\mathrm{DHW},k} &=  \dot{Q}_{\mathrm{h,DHW},k} + \dot{Q}_{\mathrm{hr,FC},k}, \label{eq:DHW_heat}
\end{align}
where all heat flows are calculated in \si{\watt}.
The sole constraint employed in this model concerns the minimum and maximum usable volumes of the storage: 

\begin{align}
  V_\mathrm{DHW,min}&\le V_{\mathrm{DHW},k} \le V_\mathrm{DHW,max}.
\end{align}

This model neglects the heat exchanger dynamics, thermal stratification, and the tap water temperature and losses are assumed to be constant.
 
%%%%%%%%%%%%%%%%%%%%%%%%%%%%%%%%%%%%%%%%%%%%%%%%%%
\subsection{Building model}\label{sec:bldg}

The thermal dynamics of the building are represented as a reduced-order building model. 
The 4R3C model is derived from \cite{langner_model_2024} and comprises three equations, which describe the indoor air dynamics, denoted by the subscript $\text{air}$, and the dynamics of internal and external temperatures of the building envelope, denoted with subscripts $\text{w,in}$ and $\text{w,out}$, respectively:

\begin{align}
    C_{\mathrm{air}} \dv{T_{\mathrm{air}}}{t} &= 
    \frac{T_{\mathrm{w,in}} - T_{\mathrm{air}}}{R_{\mathrm{w,air}}} + 
    \frac{T_{\mathrm{amb}} - T_{\mathrm{air}}}{R_{\mathrm{air,amb}}} + g_{\mathrm{s}} \dot{q}_\mathrm{s} +  f_\mathrm{conv}\dot{Q}_{\mathrm{h,SH}}, \label{eq:dT_i}\\ 
    %
    C_{\mathrm{w}} \dv{T_{\mathrm{w,in}}}{t} &= \frac{T_{\mathrm{air}} - T_{\mathrm{w,in}}}{R_{\mathrm{w,air}}} + \frac{T_{\mathrm{w,out}} - T_{\mathrm{w,in}}}{R_{\mathrm{w}}} +(1-f_\mathrm{conv})\dot{Q}_{\mathrm{h,SH}},\label{eq:dT_win}
    \\ 
    %
    C_{\mathrm{w}} \dv{T_{\mathrm{w,out}}}{t} &= \frac{T_{\mathrm{w,in}} - T_{\mathrm{w,out}}}{R_{\mathrm{w}}} + \frac{T_{\mathrm{amb,eq}} - T_{\mathrm{w,out}}}{R_{\mathrm{w,amb}}},\label{eq:dT_wout}
\end{align}

where thermal resistors are denoted by $R$s in \si{\kelvin / \watt} and indicate the insulation properties of the building. 
The thermal capacitances $C$s in \si{\joule / \kelvin} are associated with heat storage. 
The temperature nodes $T_{\mathrm{air}}$, $T_{\mathrm{w,in}}$, and $T_{\mathrm{w,out}}$ measured in \si{\kelvin}, are the indoor air, internal wall, and external wall temperatures, respectively. 
Weather-related parameters that affect the building dynamics are ambient air temperature $T_{\mathrm{amb}}$ and solar radiation $\dot{q}_\mathrm{s}$ in \si{\watt/\meter}$^2$, while $g_{\mathrm{s}}$ represents the solar heat gain factor measured in \si{\meter}$^2$. 
Variable $\dot{Q}_{\mathrm{h,SH}}$ denotes the heat flow emitted by the heat pump, $f_\mathrm{conv}$ is the convective share of heat flow, and $T_{\mathrm{amb,eq}}$ is the equivalent outdoor temperature at the exterior surfaces after accounting for solar radiation.
The set of ordinary differential equations describing the thermal dynamics of the building is reformulated into a state-space system and discretized with a zero-order hold method. 

To exploit the building thermal mass flexibility, the comfortable indoor air temperature is interpreted as the allowed temperature range at each time step $k$ described by the following equation:
\begin{equation}
    T_{\mathrm{air,min},k} \leq T_{\mathrm{air},k} \leq T_{\mathrm{air,max},k}.
\end{equation}
By maintaining the indoor air temperature within a permitted range rather than a fixed temperature set point, the controllers can use the building thermal mass as a storage to increase energy flexibility.

The model assumes uniform temperatures without air stratification.
In addition, solar gains are applied as heat input, while the internal heat gains (lighting, occupants, equipment, and related components) are neglected.


%%%%%%%%%%%%%%%% Control design%%%%%%%%%%%%
\section{\acf{CEMS} design} \label{sec:appendix}


The Mamdani fuzzy inference system \cite{mamdani1976advances} is utilized for the design of the \acp{FLC}. 
For the rule combination, the minimum function operator is chosen, while the fuzzy conclusion is derived by the maximum operator, and the defuzzification method is the center of gravity.

Figures \ref{fig:memb_functions1} and \ref{fig:memb_functions2} illustrate the inputs and outputs of the \ac{CEMS}. 
Figure \ref{fig:memb_functions1}(a) describes the membership functions of the storage states SOC and $\Delta$LOH.
Figure \ref{fig:memb_functions1}(b) illustrates thermal states, the \ac{ECDF} of the electricity price signal, and solar radiation membership functions. 
The binary describing the fuel cell toggling state is represented in Figure \ref{fig:memb_functions1}(c). 
Figures \ref{fig:memb_functions1}(d) and \ref{fig:memb_functions2}(a) depict membership functions of residual loads $\Delta P$ and $\Delta P_\mathrm{new}$ normalized on the scale of 10\,\si{k\watt}. 
To determine the membership functions, we use specific system values. 
For the peak of the ``medium negative" membership function of residual load $\Delta P$, the load that can be covered only by the fuel cell is chosen. 
For the peak of the ``big negative" membership function of residual load $\Delta P$, the load that can be covered by the fuel cell and \ac{BESS} is selected. 
The same applies to the rest of the residual load $\Delta P_\mathrm{new}$, where the ``medium positive" and the ``medium negative" peaks refer to half of the \ac{BESS} maximum power. 
Similarly, the ``big positive" and the ``big negative" upper bases of the rest of the residual load $\Delta P_\mathrm{new}$ refer to the maximal \ac{BESS} charging and discharging power, respectively. 
Figures \ref{fig:memb_functions2}(b)-(d) illustrate the membership functions of control signals: $\alpha_\mathrm{HP}$, $\alpha_\mathrm{BESS}$ and $\alpha_\mathrm{FC}$.

\begin{figure}[h]    
    \centering
    \includegraphics[width=0.8\textwidth]{figures/memb_functions_fuzzyEMS1_v3.pdf}
    \caption{Membership functions for the inputs of the \ac{CEMS}. The abbreviations in the figure are as follows: SP - small positive; MP - medium positive; BP - big positive; Z - zero; SN - small negative; MN - medium negative; BN - big negative. Variables with the subscript ``norm" are normalized to the range [0,1].}
    \label{fig:memb_functions1} 
\end{figure}

\begin{figure}[h]                     
    \centering
    \includegraphics[width=0.8\textwidth]{figures/memb_functions_fuzzyEMS2_v3.pdf}
        \caption{Membership functions for the \ac{BESS} input and control signals of the \ac{CEMS}. The abbreviations in the figure are as follows: SP - small positive; MP - medium positive; BP - big positive; Z - zero; SN - small negative; MN - medium negative; BN - big negative. Variable with the subscript ``norm" is normalized to the range [0,1].}
        \label{fig:memb_functions2}
\end{figure}


%%%%%%%%%%%%%Tabel description
Table \ref{tab:FLCflex_rules} presents a section of the FLC$_\mathrm{flex}$ rules. 
For example, suppose the state in the storage is not favorable, SOC and $\Delta$LOH indicate ``empty", solar radiation $\dot{q}_\mathrm{s}$ is ``low", and the $\hat{F}(p_\mathrm{buy})$ shows the lowest electricity prices in time step $k$ compared to day-ahead prices. 
The output $\alpha_\mathrm{HP}$ will indicate ``big positive" (see first rule in Table \ref{tab:FLCflex_rules}). 
However, if the \ac{ECDF} of electricity price signals indicates the highest prices at the time step $k$, the FLC$_\mathrm{flex}$ will work in saving mode with an output $\alpha_\mathrm{HP}=$``Z" indicating zero (see second rule in Table \ref{tab:FLCflex_rules}). 
Furthermore, if prices and solar radiation are ``high", the controller will operate the heat pump to store additional energy in the building thermal mass by increasing electrical demand (see the third rule in Table \ref{tab:FLCflex_rules}). 
The seventh rule illustrates the following conditions: the thermal state in the building is favorable, e.g., $\min(\chi_\mathrm{SH},\chi_\mathrm{DHW})$ is ``high", the hydrogen daily use indicates ``empty", SOC is ``average", \ac{ECDF} of the electricity price signal is ``high" and $\dot{q}_\mathrm{s}$ is ``low". As a result, the controller will work in saving mode, giving the output $\alpha_\mathrm{HP}=$``big negative".
This reduces the flexible thermal load because electricity prices are high, storage is not full, and indoor air temperature and usable domestic hot water volume are already approaching higher constraints. 
The control output $\alpha_\mathrm{HP}$ presents the increment or decrement of the heat pump modulation factor $\eta_\mathrm{HP}$ from the previous time step:
 %as well as external conditions $\hat{p}_\mathrm{buy}$ and $\dot{q}_\mathrm{s}$ 
\begin{align}
    \eta_{\mathrm{HP},k}=\alpha_{\mathrm{HP},k} + \eta_{\mathrm{HP},k-1}.
\end{align}
\begin{table}[h]
    \centering
    \renewcommand{\arraystretch}{1.2}
    \caption{The snapshot from FLC$_\mathrm{flex}$ rule base. The abbreviations in the table are as follows: BP - big positive; Z - zero; SP - small positive; BN - big negative.}
    \begin{tabular}{p{2cm} p{1.4cm} p{1.2cm} p{1.2cm} p{1.2cm} p{1.2cm}}
         $\min(\chi_\mathrm{SH},\chi_\mathrm{DHW})$  & $\Delta$LOH & SOC 
         & $\hat{F}(p_\mathrm{buy})$ & $\dot{q}_\mathrm{s}$ & $\alpha_\mathrm{HP}$\\
         \hline
        \centering{Low}  & Empty & Empty & Low & Low & BP \\  
        \centering{Low}  & Empty & Empty & High & Low & Z \\
        \centering{Low}  & Empty & Empty & High & High & BP \\
        \centering{Low}  & Average & Average & Average & Average & BP \\
        \centering{Low}  & Full & Full & High & Low & BP \\
        \centering{Average}  & Empty & Empty & Average & High & SP \\
       \centering{High}  & Empty & Average & High & Low & BN \\ 
    \end{tabular}
    \label{tab:FLCflex_rules}
\end{table}

\begin{table}[h]
    \centering
    \renewcommand{\arraystretch}{1.2}
    \caption{The snapshot from FLC$_\mathrm{FC}$ rule base. The abbreviations in the table are as follows: MP - medium positive; BP - big positive; SN - small negative; MN - medium negative; BN - big negative.}
    \begin{tabular}{p{1cm} p{1.2cm} p{1.2cm} p{1.2cm} p{1.2cm} p{1.2cm}}
         {\centering $\Delta P$ } & $\Delta$LOH& SOC 
          & $\hat{F}(p_\mathrm{buy})$& $s_\mathrm{on/off}$ & $\alpha_\mathrm{FC}$\\
         \hline
         \centering{SN}  & Empty & Full & High & Off & Off \\  
         \centering{SN}  & Average & Empty & Average & Off & Off \\
         \centering{SN}  & Average & Empty & Average & On & MP \\
         \centering{MN}  & Average & Empty & Low & Off & Off \\
         \centering{MN}  & Average & Empty & High & Off & BP \\
         \centering{MN}  & Full & Empty & High & Off & BP \\
         \centering{BN}  & Average & Empty & Average & On & BP \\   
    \end{tabular}
    \label{tab:FLCfc_rules}
\end{table}


Table \ref{tab:FLCfc_rules} shows part of the rule base for fuel cell operation. 
For example, the second and third rules describe situations where fuel cell operation depends on the previous state. The residual load $\Delta P$ is ``small negative", and the permissible amount of hydrogen for daily use is ``average". 
At the same time, the \ac{BESS} is empty, and the \ac{ECDF} of the electricity price signal is ``average". 
In this case, if the fuel cell was in operation, the output signal would be ``medium positive" (the third rule in Table \ref{tab:FLCfc_rules}), but if the fuel cell was not working in the previous time step, it would stay ``off" (the second rule in Table \ref{tab:FLCfc_rules}). Furthermore, if the \ac{ECDF} of the electricity price signal is ``high" but there is an ``average" or ``full" daily permissible amount of hydrogen to use $\Delta$LOH,  the fuel cell will be switched on with $\alpha_\mathrm{FC}=$``big positive" (see fifth and sixth rules). 
The control output $\alpha_\mathrm{FC}$ is multiplied by the maximal fuel cell current $I_\mathrm{FC,max}$: 
\begin{align}
    I_{\mathrm{FC},k} = \alpha_{\mathrm{FC},k} I_\mathrm{FC,max}.
\end{align}


Battery management FLC$_\mathrm{BESS}$ depends on the rest of the residual load $\Delta P_\mathrm{new}$ that needs to be covered, \ac{SOC}, and $\hat{F}(p_\mathrm{buy}$), and is presented in Table \ref{tab:FLCb_rules}. 
Suppose the \ac{SOC} indicates ``empty", $\hat{F}(p_\mathrm{buy})$ indicates ``low" and the rest of the residual load indicates ``small negative".
The output of the controller $\alpha_\mathrm{BESS}$ will define the battery charging as ``big positive", as the purchasing price is currently favorable, and the load will be purchased from the grid (see first rule):
\begin{align}
    P_{\mathrm{buy},k} = |\Delta P_{\mathrm{new},k}| + \alpha_{\mathrm{BESS},k} P_\mathrm{ch,max}.
\end{align} 

On the other hand, if the SOC is ``average" and the $\hat{F}(p_\mathrm{buy})$ is ``high", the battery will cover the residual load, and if necessary, the rest will be purchased from the grid (see fourth and sixth rule). This is defined as follows:
\begin{align}
    P_{\mathrm{d},k} &=  |\alpha_{\mathrm{BESS},k}| |\Delta P_{\mathrm{new},k}|,\\
    P_{\mathrm{buy},k} &= (1-|\alpha_{\mathrm{BESS},k}|) |\Delta P_{\mathrm{new},k}|.
\end{align}

At the end, if the rest of the residual power is positive, indicating generation, and the control signal is positive, the control signal $\alpha_{\mathrm{BESS}}$ sets the ratio of charging \ac{BESS} and selling the power to the grid (see last rule in Table \ref{tab:FLCb_rules}):
\begin{align}
    P_{\mathrm{ch},k} &= \alpha_{\mathrm{BESS},k} \Delta P_{\mathrm{new},k},\\
    P_{\mathrm{sell},k}&=(1-\alpha_{\mathrm{BESS},k}) \Delta P_{\mathrm{new},k}.
\end{align}


\begin{table}[h]
    \centering
    \renewcommand{\arraystretch}{1.2}
    \caption{The snapshot from FLC$_\mathrm{BESS}$ rule base. The abbreviations in the table are as follows: BP - big positive; SN - small negative; MN - medium negative; BN - big negative; MP - medium positive.}
    \begin{tabular}{ p{1.2cm} p{1.2cm} p{1.2cm} p{1.2cm}}
         $\Delta P_\mathrm{new}$  & SOC 
         & $\hat{F}(p_\mathrm{buy})$ & $\alpha_\mathrm{BESS}$\\
         \hline
         \centering{SN}  & Empty & Low & BP \\  
         \centering{SN}  & Empty & High & Off \\
         \centering{SN}  & Average & Low & MP \\
         \centering{MN}  & Average & High & MN \\
         \centering{BN}  & Average & Average & MN \\
         \centering{BN}  & Average & High & BN \\
         \centering{MP}  & Empty & Low & BP \\
    \end{tabular}
    \label{tab:FLCb_rules}
\end{table}

\begin{figure}[t]
    \centering
    \includegraphics[width=0.8\textwidth]{figures/FLC_3D_rules_fuzzyEMS1_v2.pdf}
    \caption{Example of the \ac{CEMS} input-output mapping: (a) FLC$_\mathrm{flex}$ when SOC $ =10\%$ and $\Delta$LOH $=10\%$, (b) FLC$_\mathrm{FC}$ under the condition of SOC~ $=20\%$  and $\Delta$LOH $= 80\%$, (c) FLC$_\mathrm{BESS}$ for SOC $ =50\%$.} 
    \label{fig:FLC_3D}
\end{figure}

Furthermore, Figure \ref{fig:FLC_3D} depicts the input-output mapping for (a) FLC$_\mathrm{flex}$, (b) FLC$_\mathrm{FC}$ and (c) FLC$_\mathrm{BESS}$. 
In the case of FLC$_\mathrm{flex}$, the SOC and $\Delta$LOH are at $10\%$. 
FLC$_\mathrm{flex}$ sets the control signal based on \ac{ECDF} electricity price signal $\hat{F}(p_\mathrm{buy})$ and current solar radiation $\dot{q}_\mathrm{s}$. 
When the electricity price signal is low or solar radiation is high, the flexible thermal load increases. 
In this way, the system stores either relatively cheap purchased energy or \ac{PV} generation in building thermal mass by increasing the indoor air temperature.
However, the indoor air temperature is controlled to remain within temperature constraints, without violating occupants' thermal comfort.
Figure \ref{fig:FLC_3D}(b) shows the situation when load and \ac{ECDF} of electricity price signals vary. 
The following inputs are kept constant: $\Delta$~LOH is $80\%$, SOC is $20\%$, and previous toggling state is on.
The figure indicates load as negative, and excess energy as positive. 
It can be concluded that as the load and the \ac{ECDF} of the electricity price signals increase, the FLC$_\mathrm{FC}$ will increase the control signal $\alpha_\mathrm{FC}$. 
If the load is under 1500\,\si{\watt} and the fuel cell is already turned on, FLC$_\mathrm{FC}$ tries to cover the load alone.
Figure \ref{fig:FLC_3D}(c) shows the case of controlling the \ac{BESS} by FLC$_\mathrm{BESS}$, when SOC is at $50\%$, where the \ac{ECDF} of the electricity price signal and the rest of the residual load are varying. 
Negative control signal $\alpha_\mathrm{BESS}$ defines the discharging state, while a positive factor defines the charging. 
As \ac{ECDF} prices are low and the load is small, $\alpha_\mathrm{BESS}$ increases.
This means the grid covers the load, and energy is purchased to charge the \ac{BESS}. 
However, as load and electricity prices increase, the FLC$_\mathrm{BESS}$ tries to discharge the \ac{BESS} as much as possible to cover the load. 


\section{Parameters}
\label{sec:appendix_parameters}

Table \ref{tab:parameters_PV_batt_dhw_h2} provides the parameters used to dimension \ac{PV}, \ac{BESS}, domestic hot water storage, and hydrogen systems.
The parameters used for the \ac{PV} model are as follows: number of modules $n_\mathrm{module}$, area of one module $a_\mathrm{module}$, nominal operating cell temperature $NOCT$, temperature under the standard testing conditions $T_\mathrm{STC}$, electrical efficiency under standard testing conditions $\eta_\mathrm{STC}$, combined inverter and maximum power point tracking losses $\eta_\mathrm{L\&T}$, and temperature coefficient $\eta_\mathrm{T}$.
For \ac{BESS}, the following parameters and initial values are provided: maximum energy capacity $E_\mathrm{B,max}$, maximal charging and discharging power $P_\mathrm{ch,max}$ and $P_\mathrm{d,max}$, respectively, charging and discharging efficiencies $\eta_\mathrm{ch}$ and $\eta_\mathrm{d}$, respectively, and maximal, minimal and initial state of charge SOC$_\mathrm{max}$, SOC$_\mathrm{min}$ and SOC$_\mathrm{init}$, respectively. 
In the domestic hot water storage model, the following parameters are defined: maximal and minimal storage volume $V_\mathrm{DHW,max}$ and $V_\mathrm{DHW,min}$, respectively, standing losses $\dot{Q}_\mathrm{l,DHW}$ and temperature of usable hot water in the storage $T_\mathrm{DHW}$.
Furthermore, for the hydrogen system, the following parameters are provided: maximal and minimal current $I_\mathrm{FC,max}$ and $I_\mathrm{FC,min}$, respectively, active area of the stack $a_\mathrm{cell}$, number of the cells $n_\mathrm{cell}$, cogeneration efficiency $\eta_\mathrm{FC,sys}$, maximal current density $i_\mathrm{FC,max}$, maximal energy stored $E_\mathrm{H_2,max}$ and initial level of hydrogen in the storage LOH$_\mathrm{init}$.
\begin{table}[htbp!]
    \centering
    \renewcommand{\arraystretch}{1.1}
    \newcolumntype{C}[1]{>{\centering\arraybackslash}p{#1}}
    \caption{\ac{PV}, \ac{BESS}, domestic hot water storage and hydrogen system parameters.}
    \begin{tabular}{C{2.0cm}| C{1.5cm} C{2cm} C{1.5cm} C{1.5cm}}

         \centering{Component} & Variable & Value 
         & Variable & Value \\
         \hline
         \multirow{4}{4em}{\centering PV} & $n_\mathrm{module}$  & 30& $\eta_\mathrm{STC}$ & 0.19 \\  
         & $a_\mathrm{module}$ & 1.685\,$\si{\meter}^2$ & $NOCT$ & 50 \si{\degree C}   \\ 
         & $\eta_\mathrm{T}$ & 0.005\,$\si{\degree C}^{-1}$ & $T_\mathrm{STC}$ &25\,\si{\degree C}   \\ 
         & $\eta_\mathrm{L\&T}$ & 0.9&  &    \\ 
         \hline
         \multirow{4}{4em}{\centering \ac{BESS}} & $E_\mathrm{B,max}$  & 4.8\,\si{k\watt\hour}& $P_\mathrm{d,max}$ & 2880\,\si{\watt} \\  
         & $\eta_\mathrm{ch}$ & 0.93 & SOC$_\mathrm{min}$& 10\%   \\ 
         & $\eta_\mathrm{d}$ & 0.93 & SOC$_\mathrm{max}$& 90\%   \\ 
         & $P_\mathrm{ch,max}$ &2880\,\si{\watt}& SOC$_\mathrm{init}$  & 50\%    \\ 
         \hline
          \multirow{2}{6.5em}{\centering Domestic hot water storage} & $V_\mathrm{DHW,max}$  & 300\,\si{litres}& $V_\mathrm{DHW,min}$  & 40\,\si{litres} \\
          & $\dot{Q}_\mathrm{l,DHW}$  & 35\,\si{\watt}& $T_\mathrm{DHW}$  & 45\,\si{\degree C}\\
          \hline
          \multirow{3}{5em}{\centering Hydrogen system} &  $I_\mathrm{FC,max}$  & 180\,\si{\ampere}& $I_\mathrm{FC,min}$ & 50\,\si{\ampere} \\  
          &$a_\mathrm{cell}$  & 200 \si{cm}$^2$  & $\eta_\mathrm{FC,sys}$ & 0.75 \\
          &$n_\mathrm{cell}$
            & 22& i$_\mathrm{FC,max}$  & 1.6\,$\si{\ampere/cm}^2$  \\
          &$E_\mathrm{H_2,max}$
            & 1800 \si{k\watt \hour}& LOH$_\mathrm{init}$  & 100\%  \\
    \end{tabular}
    \label{tab:parameters_PV_batt_dhw_h2}
\end{table}


Table \ref{tab:degradation_HESS} presents the degradation costs for the hybrid energy storage system, where $\sigma_\mathrm{in,FC}$ and $\sigma_\mathrm{in,BESS}$  in~\si{\EUR} represent the initial investment costs of the fuel cell and \ac{BESS}, respectively. 
The lifespan of the fuel cell is defined as $L_\mathrm{FC}$, while operational and maintenance costs of the fuel cell are defined as $\sigma_\mathrm{om,FC}$.
The lifetime of the \ac{BESS} cannot be found directly in datasheets, but rather needs to be calculated based on the depth-of-discharge cycles $N_\mathrm{BESS}$. 
The lifespan can then be calculated as described in \cite{cau2014energy}. The above-mentioned investment costs, fuel cell lifespan, and depth-of-discharge cycles $N_\mathrm{BESS}$ are based on the datasheets of corresponding components \cite{battery_costs,FC_costs}.
The operation and maintenance costs for the \ac{BESS} are assumed to be negligible, while those for the fuel cell are defined in \cite{wang_mpc-based_2024}. 
Furthermore, the ON/OFF costs of the hydrogen components are defined with $\sigma_\mathrm{FC,on}$ and $\sigma_\mathrm{FC,off}$. %The letter two costs of the \ac{HESS} are further derived from \cite{wang_mpc-based_2024}. 

%%%without EL
\begin{table}[h]
    \centering
    \renewcommand{\arraystretch}{1.2}
    \caption{Degradation costs of the energy storage systems. Investment costs, fuel cell lifespan, and depth-of-discharge cycles of \ac{BESS} are based on  \cite{battery_costs,FC_costs}, while fuel cell operation and maintenance costs are based on \cite{wang_mpc-based_2024}.}
    \newcolumntype{C}[1]{>{\centering\arraybackslash}p{#1}}
    \begin{tabular}{C{2cm}| C{1.5cm} C{2cm} C{1.5cm} C{2cm}}
          Component & Variable & Value 
         & Variable & Value \\
         \hline
         \multirow{3}{4em}{Fuel cell} &  $\sigma_\mathrm{in,FC}$  & 10908\,\si{\EUR} & $\sigma_\mathrm{om,FC}$
            & 0.038\,\si{\EUR/\hour} \\  
          & $L_\mathrm{FC}$  & 35000\,\si{\hour} & $\sigma_\mathrm{FC,on}$ & 0.10\,\si{\EUR} \\
          & $\sigma_\mathrm{FC,off}$ & 0.053\,\si{\EUR} & & \\
          \hline
          \ac{BESS} & $\sigma_\mathrm{in,BESS}$
          & 900\,\si{\EUR}& $N_\mathrm{BESS}$ & 6000 cycles \\
    \end{tabular}
    \label{tab:degradation_HESS}
\end{table}
